# Supplementary material for: GNN-MultiFix: Addressing the pitfalls for GNNs for multi-label node classification
Source: arXiv:2411.14094 source file (2024-11-21)
Supplement: Supplementary file 1 [file additionalanalysis.tex]

\subsection{Additional analysis of \mymodel}
 The experiments are designed to answer the following research questions: (i) Does different modules in \mymodel provide useful information for the node classification task?

\subsubsection{Modules In \mymodel}
\label{app:modules}
To answer the first question of the information provided by the positional embeddings, we load \mymodellin trained on one split of the \blog dataset and visualize the learned weights $\mathbf{W}$ in the last fusion layer using heatmap in Figure \ref{fig:weights_all}. As all non-linearity is removed in \mymodellin, the learned weights can be seen as the importance assigned by the model to the different parts of our model, we visualize the weights for feature representation in Subfigure \ref{fig:weights_fp}, label representation in Subfigure \ref{fig:weights_lp}, and positional representation in Subfigure \ref{fig:weights_pe}.

Since we concatenate $\mathbf{h}^{(K)}_{f_v} \in \mathbb{R}^{n \times \text{hidden\_dim}}$, $\mathbf{h}^{(N)}_{l_v} \in \mathbb{R}^{n \times C}$, and $\mathbf{\phi}_v \in \mathbb{R}^{n \times \text{PE\_dim}}$ as the input of the fusion layer, we denote $H = \text{hidden\_dim} + C + \text{PE\_dim}$, thus $\mathbf{W} \in \mathbb{R}^{C \times H}$ and the weights learned for feature representation, label representation, and positional representation have the shape of $\mathbf{W}_{f_v} \in \mathbb{R}^{C \times \text{hidden\_dim}}$, $\mathbf{W}_{l_v} \in \mathbb{R}^{C \times C}$, and $\mathbf{W}_{\phi_v} \in \mathbb{R}^{C \times \text{PE\_dim}}$ respectively.

In our visualization, the darker the cell is, the higher the weights are. However, small negative weights learned by the model can also be meaningful, indicating negative correlations between the input and output. Thus, the more contrastive the weights are, the more important are the part of the input for the output. 

% As shown in Figure \ref{fig:weights_visualization}, in the dataset without input features, our model learns to focus on the positional embedding to break the graph isomorphism and generate different embeddings for similar nodes, thus enhance the expression ability of graph neural networks.

\begin{figure}[!h]
    \centering
    \begin{subfigure}{0.48\textwidth}
        \includegraphics[width=\textwidth]{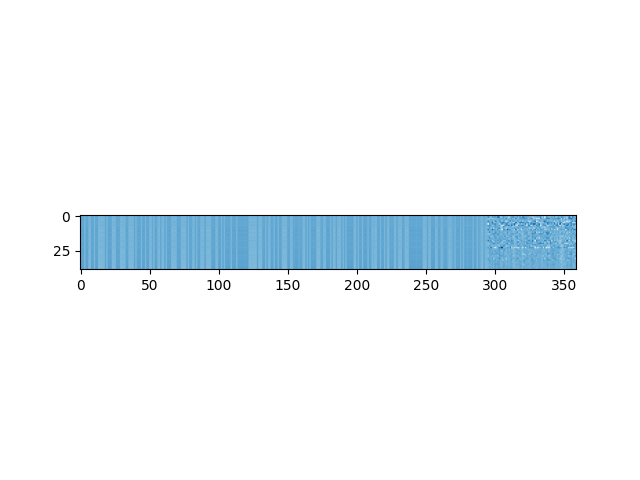}
        \caption{Visualization of weights in the fusion layer of our linear model on \blog.}
        \label{fig:weights_all}
    \end{subfigure}
    \hfill
    \begin{subfigure}{0.48\textwidth}
        \includegraphics[width=\textwidth]{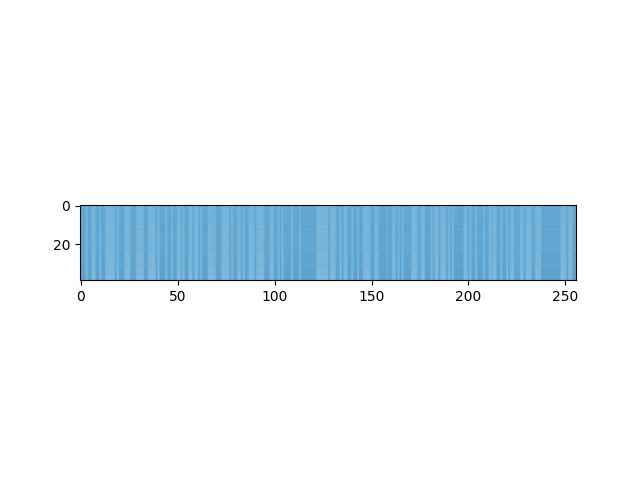}
        \caption{Visualization of weights in the linear model for feature propagation on \blog.}
        \label{fig:weights_fp}
    \end{subfigure}
    \hfill
    \begin{subfigure}{0.48\textwidth}
        \includegraphics[width=\textwidth]{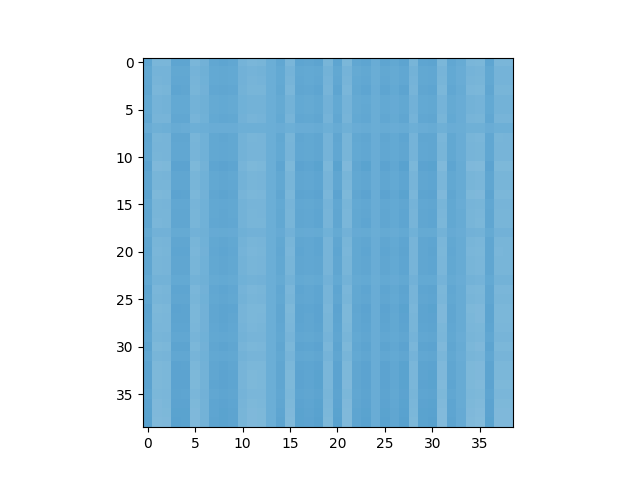}
        \caption{Visualization of weights in the linear model for label propagation on \blog.}
        \label{fig:weights_lp}
    \end{subfigure}
    \hfill
    \begin{subfigure}{0.48\textwidth}
        \includegraphics[width=\textwidth]{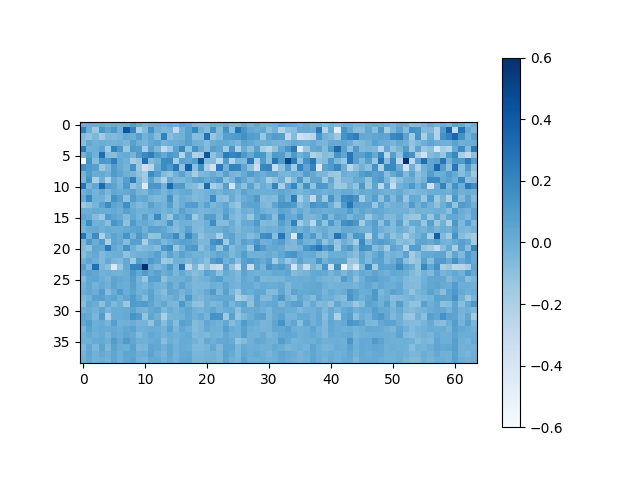}
        \caption{Visualization of weights in the linear model for positional representation on \blog.}
        \label{fig:weights_pe}
    \end{subfigure}
    \caption{Visualization of weights in the fusion layer of \mymodellin trained on \blog dataset. All the subplots use the same value bar as in \ref{fig:weights_pe}.}
    \label{fig:weights_visualization}
\end{figure}

\begin{figure}[!h]
    
    \begin{subfigure}{0.49\textwidth}
        \includegraphics[width=\textwidth]{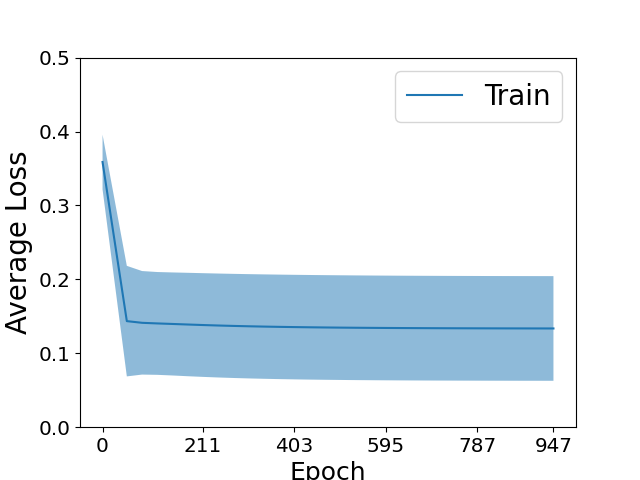}
        \caption{\mymodellin on the \blog dataset.}
    \end{subfigure}
    \hfill
    \begin{subfigure}{0.47\textwidth}
        \includegraphics[width=\textwidth]{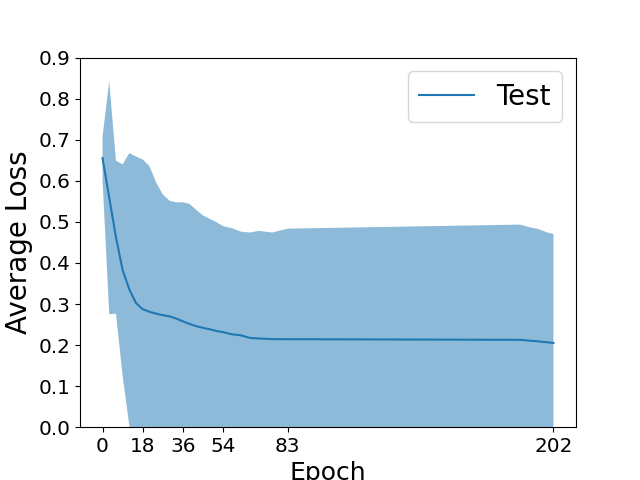}
        \caption{\mymodellin on the \dblp dataset.}
    \end{subfigure}
    \caption{Visualization of the training loss of \mymodellin on the \blog and \dblp dataset. Captions of the subfigure marks the name of the model and the dataset. }
    \label{fig:train_dym}
\end{figure}

\subsubsection{Homophily Recovery}
\label{app:recover_homo}
\begin{wrapfigure}{r}{0.5\textwidth}
\vspace{-50pt} 
  \begin{center}
    \includegraphics[width=0.4\textwidth]{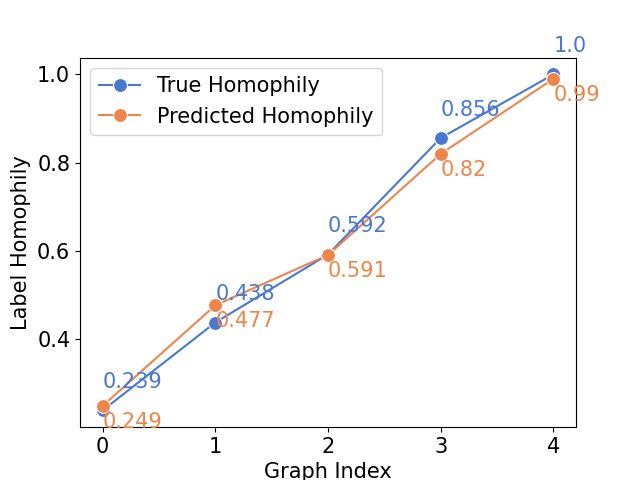}
  \end{center}
  \caption{The label homophily predicted for \homolevel by \mymodelMlp and the true label homophily.}
  \label{fig:homophily}
  \vspace{-20pt}
\end{wrapfigure}

We use \mymodelMlp trained for the varying homophily experiment on the five synthetic datasets with varying label homophily. We use $0.5$ as a threshold to convert the output probabilities of our model into predictions and calculate the label homophily of the predicted graph. The label homophily levels of the predicted graph and the original graph are summarized in the Figure \ref{fig:homophily}. As shown in the figure, our model successfully recovers the label homophily in the input graph.
